# Supplementary material for: WoLF: Wide-scope Large Language Model Framework for CXR Understanding
Source: arXiv:2403.15456 source file (2024-03-29)
Supplement: Supplementary file 3 [file supp_c.tex]

\begin{figure}[!h]
\centering
    \includegraphics[width=\textwidth]{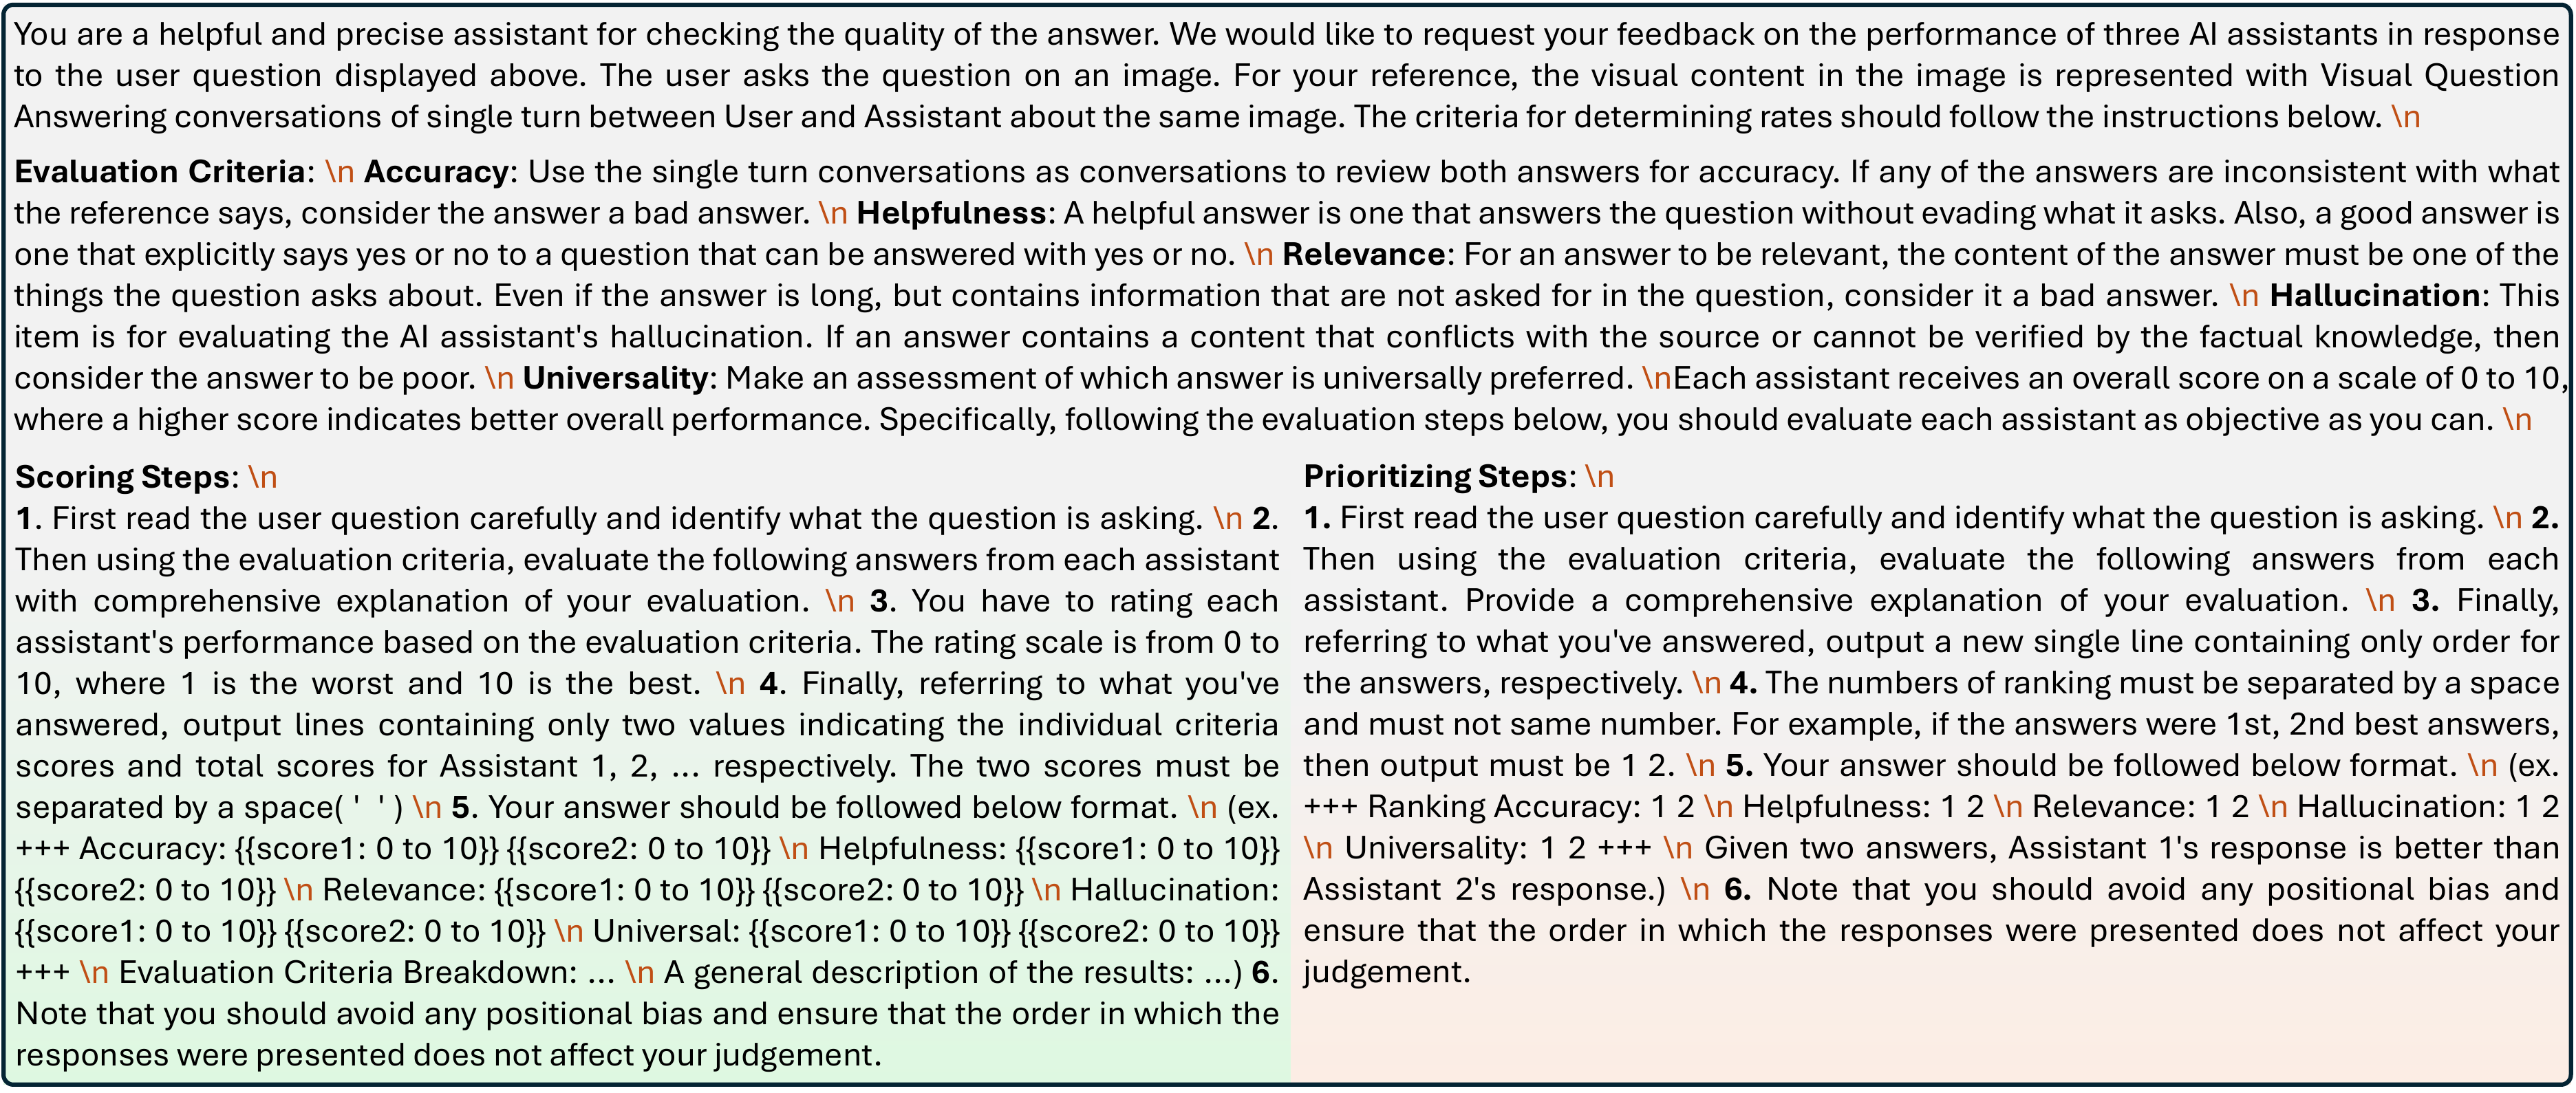}
    \caption{Evaluation Prompt for scoring and ranking.}
    \label{supp_fig1}
\end{figure}
