# Supplementary material for: WoLF: Wide-scope Large Language Model Framework for CXR Understanding
Source: arXiv:2403.15456 source file (2024-03-29)
Supplement: Supplementary file 4 [file supp_d.tex]

\begin{figure}[h]
    \centering
    \scalebox{0.86}{
    \begin{tabular}{c}
        \includegraphics[width=\textwidth]{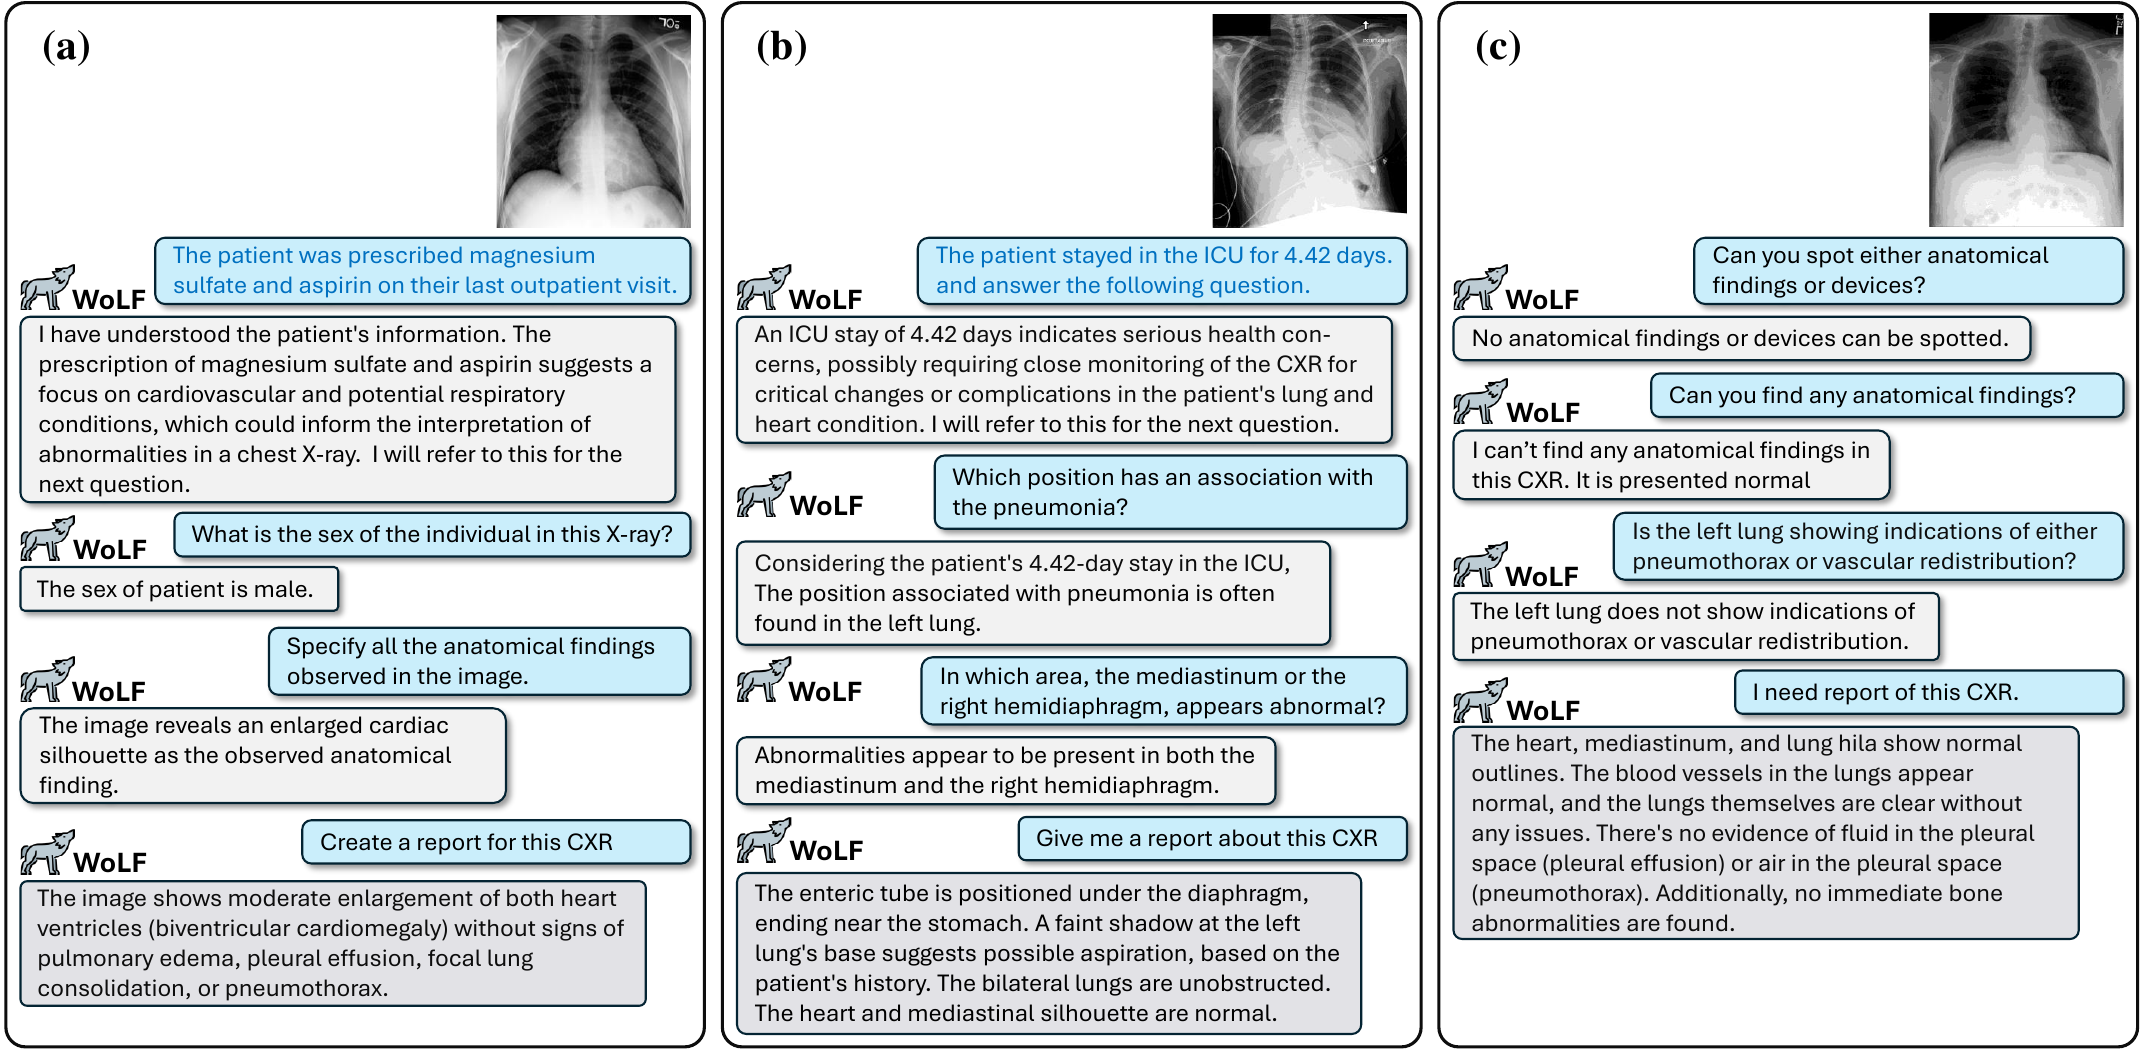}
        
    \end{tabular}
    }
    \caption{Qualitative results of visual question-answering scenarios. In (a) and (b), we feed models with patient histories and medication details from EHRs. WoLF utilizes this to deliver more accurate responses.}\
    \label{tab:my_label}
\end{figure}
